# Supplementary material for: Construction of Chemistry Inspired Dynamic Ansatz Utilizing Generative Machine Learning
Source: arXiv:2503.08149 ancillary file (2025-03-11)
Supplement: Supplementary file 1 [file Supplementary_Information.pdf]

# Supporting Information

## Construction of Chemistry Inspired Dynamic Ansatz Utilizing Generative Machine Learning

*Sonaldeep Halder*[†], *Kartikey Anand*[†], *and Rahul Maitra*[*,†,‡]

[†]Department of Chemistry, Indian Institute of Technology Bombay, Powai, Mumbai 400076, India

[‡]Centre of Excellence in Quantum Information, Computing, Science & Technology, Indian Institute of Technology Bombay, Powai, Mumbai 400076, India

**Corresponding Author**

* E-mail address: rmaitra@chem.iitb.ac.in

**S1. Implementation of a disentangled Unitary Coupled Cluster (dUCC) Ansatz using quantum circuits**

A disentangled unitary coupled cluster ansatz can be written as:

$$\hat{U}(\theta) = \prod_{\mu} e^{\theta_{\mu}\hat{\kappa}_{\mu}}$$

$$\hat{\kappa}_{\mu} = \hat{\tau}_{\mu} - \hat{\tau}_{\mu}^{\dagger}$$

$$\hat{\tau}_{\mu} = \hat{a}_{p}^{\dagger}\hat{a}_{q}^{\dagger}..........\hat{a}_{r}\hat{a}_{s}$$

Here, p,q,...,r,s are general orbital indices $\hat{a}^{\dagger}$ and $\hat{a}$ are fermionic creation and annihilation operators respectively. dUCC ansatz may consist of “true” excitations, that is, {p,q,...} belong to unoccupied orbital indices and {r,s,..} belong to occupied ones. As discussed in the next section of this supplementary information, the scatterer operators are also used in the manuscript. They can contain unoccupied to unoccupied and occupied to occupied “excitations.” Thus, to consider such “excitations” as well, a general notation of orbital indices {p,q,...,r,s} is used. Here, these indices can mean either an occupied or unoccupied orbital.

The fermionic creation and annihilation operators can be converted to quantum gates using some mapping techniques. The Jordan-Wigner mapping[1] used in the manuscript is defined as:

$$\hat{a}_p^{\dagger} = \frac{1}{2}(X_p - iY_p) \otimes Z_{p-1} \otimes Z_{p-2} \otimes ....... \otimes Z_1$$

$$\hat{a}_p = \frac{1}{2}(X_p + iY_p) \otimes Z_{p-1} \otimes Z_{p-2} \otimes ....... \otimes Z_1$$

Here, X, Y, and Z are the Pauli operators. Using this transformation, the ansatz $\hat{U}(\theta)$ can be written as a product of exponentiated Pauli operators-

$$\hat{U}(\theta) = \prod_{\nu} e^{i\theta_{\nu} P_{\upsilon}}$$

$P_{\nu}$ is a Pauli string. An exponentiated Pauli string can be implemented in quantum hardware using one and two-qubit gates[1]. For example, a circuit implementation of some terms are as follows:

a) $e^{-i(\theta)Z_3 Z_2 Z_1 Z_0}$

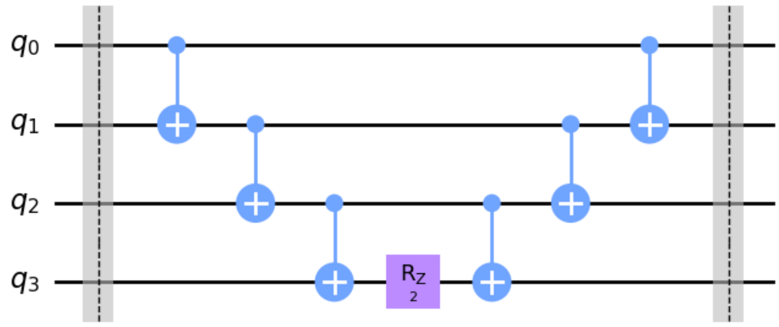


b) $e^{-i(\theta)Z_3 Z_2 Z_1 X_0}$

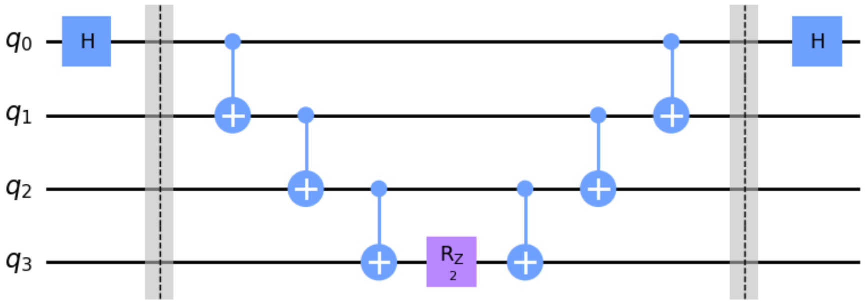


c) $e^{-i(\theta)Z_3Z_2Z_1Y_0}$

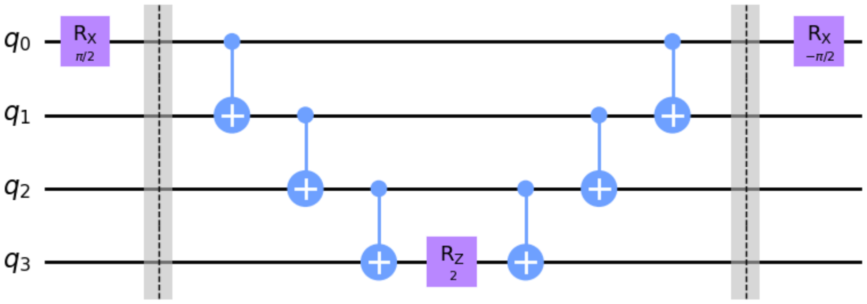


d) $e^{-i(\theta)Z_3X_2Y_1Y_0}$

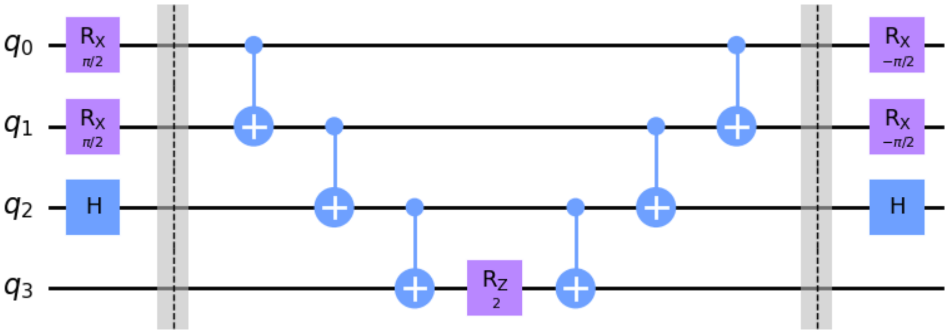


Figure. S1: Circuit Implementation using one qubit (H, $S^{\dagger}$, S and $R_Z(\omega)$) and two-qubit CNOT gates. Here $\theta = 1$ such that $\omega = 2\theta = 2$.

## S2. Decomposition of a high-rank excitation operator into a low-rank operator and a *Scatterer*

A *scatterer* is an effective one-body excitation operator with one true occupied to unoccupied excitation index and another occupied to occupied or unoccupied to unoccupied index. Diagrammatically, this can be represented as:

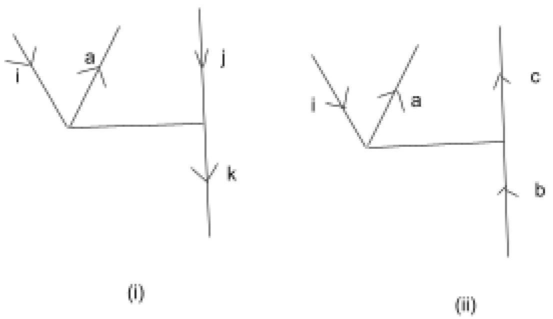


Figure. S2: A diagrammatic representation of scatterers

In Figure. S2, (i) represents the anti-hermitian scatterer $\hat{\sigma}_{ij}^{ak}$ = $\hat{a}_a^\dagger \hat{a}_k^\dagger \hat{a}_j \hat{a}_i - \hat{a}_i^\dagger \hat{a}_j^\dagger \hat{a}_k \hat{a}_a$ and (ii) represents $\hat{\sigma}_{ib}^{ac}$ = $\hat{a}_a^\dagger \hat{a}_c^\dagger \hat{a}_b \hat{a}_i - \hat{a}_i^\dagger \hat{a}_b^\dagger \hat{a}_c \hat{a}_a$. The labels i,j, and k represent occupied orbital, and a,b, and c represent unoccupied ones. $\hat{a}^\dagger$ and $\hat{a}$ are fermionic creation and annihilation operators, respectively. A high-rank excitation operator, say triples, can be produced as follows:

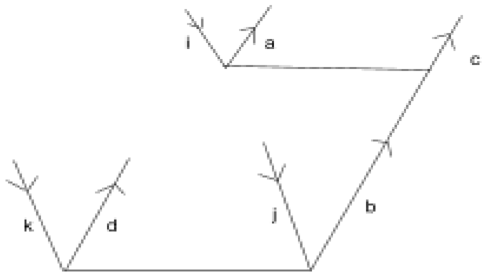


Figure. S3: A diagrammatic representation of the decomposition of high-rank excitation operators into a low-rank operator and a *scatterer*.

Thus, the anti-hermitian triples excitation operator $\hat{\kappa}_{ijk}^{acd}$ can be generated by the commutator - $[\hat{\sigma}_{ib}^{ac}, \hat{\kappa}_{kj}^{db}]$. In forming RBM1s-dUCCSDT$_S$ ansatz, we take the exponentiated form of these anti-hermitian operators. The commutator occurs as follows[2,3]:

$$e^{\hat{\sigma}} e^{\hat{\kappa}} = e^{(\hat{\sigma} + \hat{\kappa}) + \frac{1}{2}[\hat{\sigma}, \hat{\kappa}] + \ldots}$$

Thus, using a sequence of exponentiated operators of a low-rank operator and a *scatterer*, we can produce the effect of a high-rank excitation operator.

## S3. Tree-structured Parzen Estimator for hyperparameter optimization

Bayesian Hyperparameter Optimization (BHO) [4],[5],[6], particularly through the Tree-structured Parzen Estimator (TPE) [7] algorithm, significantly reduces computational costs by incorporating prior knowledge and dynamically updating the search strategy based on observed performance. TPE models the objective function—here, the ground state energy obtained using the RBM1s-dUCC ansatz—as a probabilistic distribution, E(x), where x represents the hyperparameter configuration.

The algorithm constructs two density functions: *l*(x) and *g(x).* Here, *l(x)* represents the density of hyperparameters that yield objective function values below a threshold, $y^*$, while *g(x)* corresponds to the density of hyperparameters yielding values above this threshold. The hyperparameters considered include the number of hidden nodes, the number of Gibbs sampling steps, the learning rate, and batch size.

The threshold $y^*$ is typically chosen such that a certain fraction, γ, of the observed samples fall below it:

$$y^* = \text{Quantile}\,(E(x), \gamma)$$

The expected improvement (EI) criterion is employed to evaluate the next hyperparameter configuration, x. The EI is calculated as:

$$\text{EI}(x) = \int_{-\infty}^{y^*} (y^* - y)\, p(y \mid x)\, dy$$

In the context of TPE, the probability $p(y \mid x)$ can be re-expressed using Bayes' theorem:

$$p(y \mid x) = \frac{p(x \mid y)\, p(y)}{p(x)}$$

Given the densities *l(x)* and *g(x)*, the acquisition function can be derived by maximizing the ratio $\frac{l(x)}{g(x)}$. This ratio effectively prioritizes hyperparameter configurations that are more likely to yield better performance.

$$x_{next} = \underset{x}{argmax}\, \frac{l(x)}{g(x)}$$

By focusing on regions of the hyperparameter space with higher potential for improvement, the TPE algorithm efficiently navigates the search space, minimizing the number of required evaluations and reducing computational expense.

In this work, we utilize the Optuna framework[8] for hyperparameter optimization and visually representing the obtained results. In general, this set will vary from molecule to molecule. However, as demonstrated in the main article, the same set of hyperparameters gives accurate results for different molecular systems having similar sizes (number of orbitals in a given basis). In Figure. S4, we showcase the sequential improvement in the energy during the Bayesian optimization procedure performed using TPE for the molecular system of $CH_2$ at a stretched geometry of 1.75 x $r_{eq}$ ($r_{eq}$ = 1.109 Å) and bond angle of 102.400°. The RBM is constructed using the Scikit-learn package[9]. The training uses 10000 data points with the frequency of different determinants governed by the process illustrated in Step 2 in the main article. As the optimization is stochastic, the objective function value does not decrease monotonically. However, TPE learns from each set and eventually produces a set that gives lower energy through an optimum construction of RBM1s-dUCCSDT$_{S.}$

Figure. S5 gives the values of different hyperparameters at which the energy values were obtained during the optimization. The lowest energy is obtained using 23 hidden nodes. At this optimum range, the hidden layer accurately captures the patterns within the initial approximate wavefunction to generate dominant excited determinants. The optimum number of Gibbs sampling comes at 20. Once the set of optimum hyperparameters is obtained, the RBM can efficiently generate the shallow depth ansatz to produce accurate ground state energies.

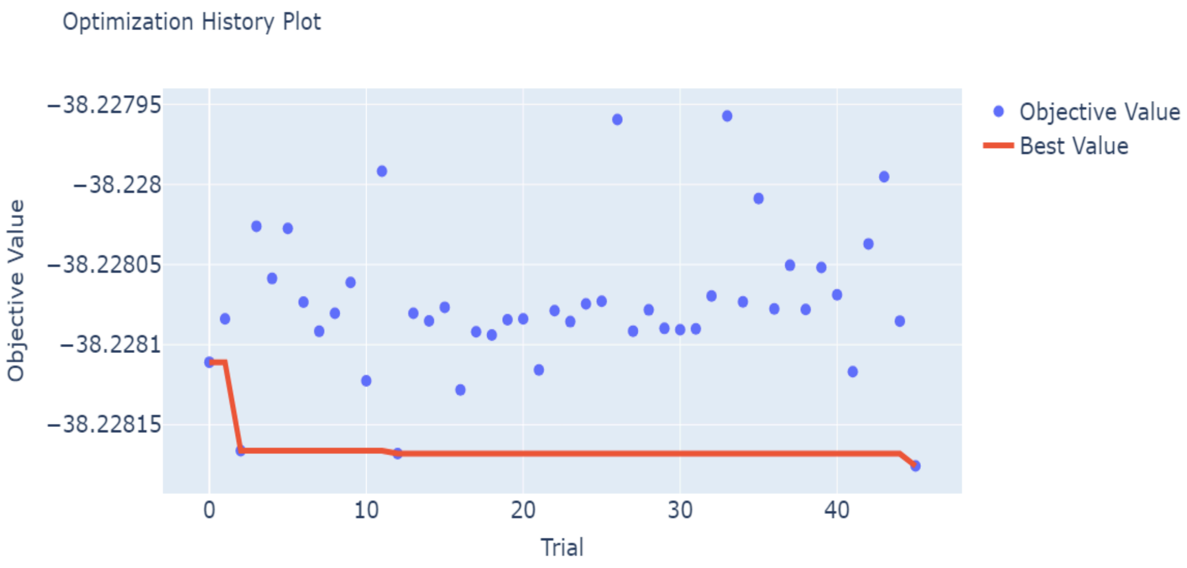


Figure. S4: The energies (objective values) obtained during the search performed by TPE during the optimization of hyperparameters

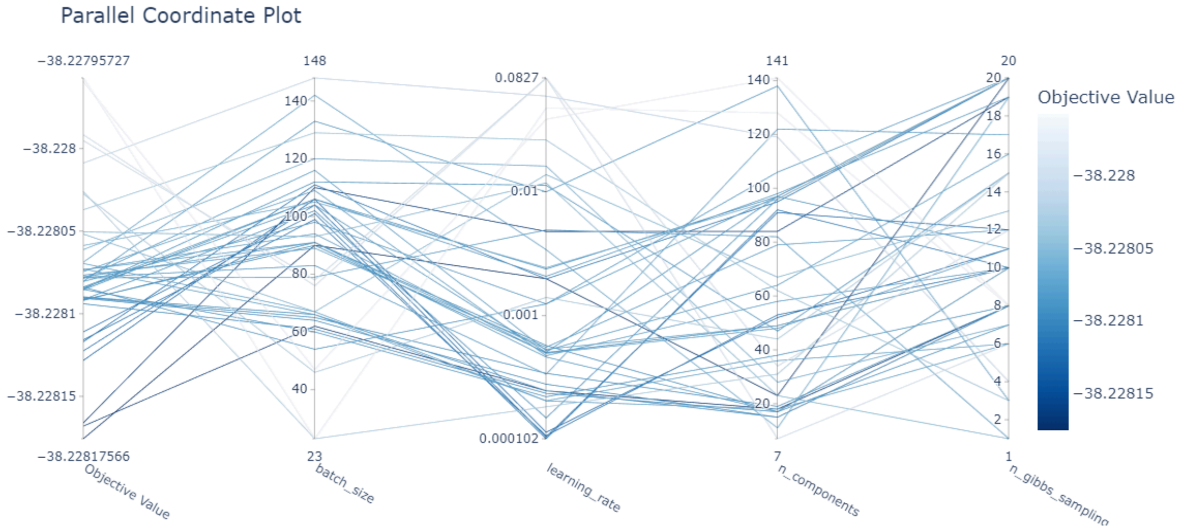


Figure. S5: Energies (objective values) obtained at different sets of the hyperparameters – (batch size, learning rate, number of hidden nodes, number of Gibbs sampling).

## S4. Optimization of RBM1s-dUCCSDTs ansatz: MP2 Vs Zero

In this section, we compare the converged energies for RBM1s-dUCCSDTS ansatz using CG optimizer (maximum iterations set to 10000) for different C-H bond stretches of $CH_2$ using two different initial points

(i) MP2 values for the doubles excitation operators and scatterers in the ansatz (singles
excitation operators are started with zero).

(ii) All parameters started with zero.

| $r_{C-H}$ (Å); ∠H-C-H = 102.400° | (i) | (ii) |
|---|---|---|
| 1.38625 | -38.392053 ($E_h$) | -38.392053 ($E_h$) |
| 1.52488 | -38.347828 ($E_h$) | -38.347828 ($E_h$) |
| 1.66350 | -38.302813 ($E_h$) | -38.302813 ($E_h$) |
| 1.80212 | -38.262037 ($E_h$) | -38.262037 ($E_h$) |
| 1.94075 | -38.228175 ($E_h$) | -38.228174 ($E_h$) |

## S5. Comparison with ADAPT-VQE

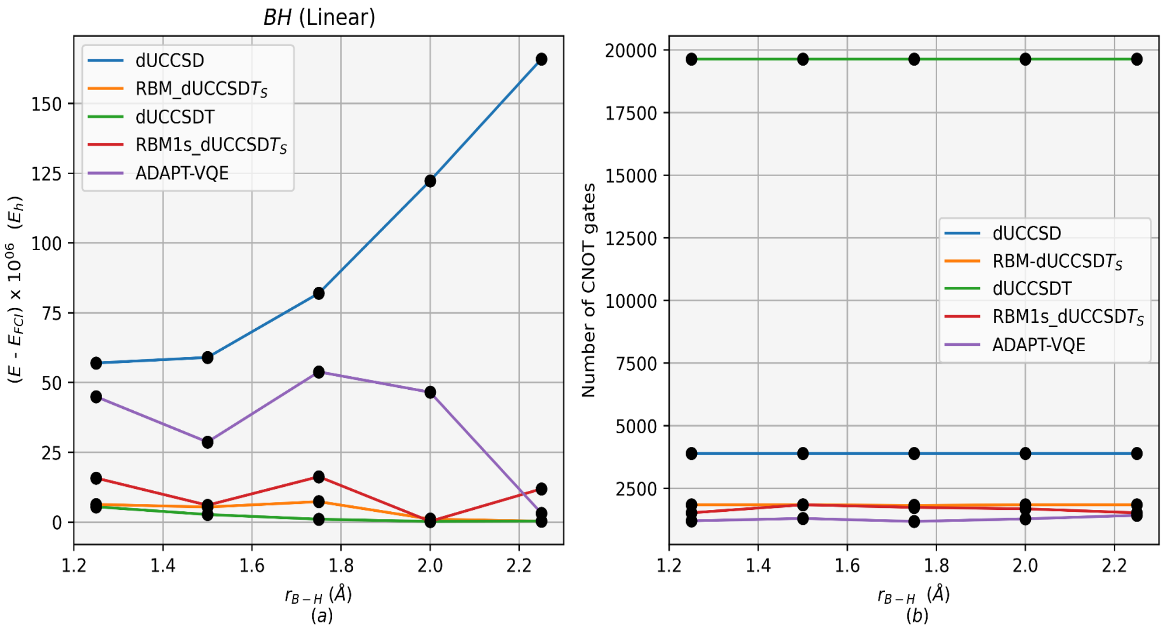

Figure. S6: Comparison of energy accuracy (with Full Configuration Interaction or FCI) and number of CNOT gates for various methods for BH (STO-3G, core orbitals frozen)

In this section, we provide a comparison of the developed method (RBM1s-dUCCSDT$_S$) with ADAPT-VQE[10], which is a well-known method for dynamic construction of shallow depth ansatz. The operator pool chosen for ADAPT-VQE is composed of generalized singles and doubles. From Fig. S6, it can be seen that the number of CNOT gates for the RBM1s-dUCCSDT$_S$ is relatively higher than ADAPT-VQE (by ≅500). However, RBM1s-dUCCSDT$_S$ has an energy error lower than ADAPT-VQE.

References:

[1] Y. Cao, J. Romero, J. P. Olson, M. Degroote, P. D. Johnson, M. Kieferová, I. D. Kivlichan, T. Menke, B. Peropadre, N. P. Sawaya, et al., “Quantum chemistry in the age of quantum computing,” Chemical reviews 119, 10856–10915 (2019).

[2] D. Halder, V. S. Prasannaa, and R. Maitra, “Dual exponential coupled cluster theory: Unitary adaptation, implementation in the variational quantum eigensolver framework and pilot applications,” The Journal of Chemical Physics **157**, 174117 (2022).

[3] N. Hatano and M. Suzuki, in *Quantum Annealing and Other Optimization Methods*, Lecture Notes in Physics Vol. **679**, edited by A. Das and B. K. Chakrabarti (Springer, 2005), pp. 36–68.

[4] J. Snoek, H. Larochelle, and R. P. Adams, “Practical bayesian optimization of machine learning algorithms,” Advances in neural information processing systems **25** (2012).

[5] J. Bergstra and Y. Bengio, “Random search for hyper-parameter optimization.” Journal of machine learning research **13** (2012).

[6] J. Bergstra, D. Yamins, and D. Cox, “Making a science of model search: Hyperparameter optimization in hundreds of dimensions for vision architectures,” in International conference on machine learning (PMLR, 2013) pp. 115–123.

[7] J. Bergstra, R. Bardenet, Y. Bengio, and B. Kégl, “Algorithms for hyper-parameter optimization,” Advances in neural information processing systems **24** (2011).

[8] T. Akiba, S. Sano, T. Yanase, T. Ohta, and M. Koyama, “Optuna: A next-generation hyperparameter optimization framework,” in Proceedings of the 25th ACM SIGKDD International Conference on Knowledge Discovery and Data Mining (2019).

[9] F. Pedregosa, G. Varoquaux, A. Gramfort, V. Michel, B. Thirion, O. Grisel, M. Blondel, P. Prettenhofer, R. Weiss, V. Dubourg et al., “Scikit-learn: Machine learning in python,” the Journal of machine Learning research **12**, 2825–2830 (2011).

[10] H. R. Grimsley, S. E. Economou, E. Barnes, and N. J. Mayhall, “An adaptive variational algorithm for exact molecular simulations on a quantum computer,” Nature communications **10**, 3007545 (2019).
